# Supplementary material for: Enhancing Heterogeneous Multi-Agent Cooperation in Decentralized MARL via GNN-driven Intrinsic Rewards
Source: arXiv:2408.06503 source file (2026-03-12)
Supplement: Supplementary file 1 [file Supplementary_Materials_Configuration_Parameters.pdf]

# Configurations Parameters and Model Hyper-parameters

**Article Title:** Decentralized Cooperation in Heterogeneous Multi-Agent Reinforcement Learning via Graph Neural Network-Based Intrinsic Motivation

**Authors:** Jahir Sadik Monon (Corresponding Author), Deeparghya Dutta Barua and Md. Mosaddek Khan

**Affiliation:** Department of Computer Science and Engineering, University of Dhaka, Bangladesh

**E-mail address of the corresponding author:** jahirsadikmonon@gmail.com

## Python Requirements for Running the Project

```
# requirements.txt for running the projects on local machine
numpy==1.23.5
vmas
wandb
torch
torch_geometric
torch_scatter
torch_sparse
torch_cluster
torch_spline_conv
```

## Anaconda Package Dependencies

```
# environment.yml for running the projects on local machine
channels:
  - defaults
dependencies:
  - abseil-cpp=20211102.0=hc377ac9_0
  - bzip2=1.0.8=h620ffc9_4
  - c-ares=1.19.0=h80987f9_0
  - ca-certificates=2023.05.30=hca03da5_0
  - grpc-cpp=1.48.2=hc60591f_1
  - grpcio=1.48.2=py310hc60591f_1
  - libcxx=14.0.6=h848a8c0_0
  - libffi=3.4.4=hca03da5_0
  - libprotobuf=3.20.3=h514c7bf_0
  - ncurses=6.4=h313beb8_0
  - openssl=3.0.9=h1a28f6b_0
  - pip=23.2.1=py310hca03da5_0
  - python=3.10.12=hb885b13_0
  - re2=2022.04.01=hc377ac9_0
  - readline=8.2=h1a28f6b_0
  - setuptools=68.0.0=py310hca03da5_0
```

```
- six=1.16.0=pyhd3eb1b0_1
- sqlite=3.41.2=h80987f9_0
- tk=8.6.12=hb8d0fd4_0
- wheel=0.38.4=py310hca03da5_0
- xz=5.4.2=h80987f9_0
- zlib=1.2.13=h5a0b063_0
- pip:
  - aiosignal==1.3.1
  - amqp==5.1.1
  - appdirs==1.4.4
  - attrs==23.1.0
  - billiard==4.1.0
  - celery==5.3.1
  - certifi==2023.7.22
  - charset-normalizer==3.2.0
  - click==8.0.4
  - click-didyoumean==0.3.0
  - click-plugins==1.1.1
  - click-repl==0.3.0
  - cloudpickle==2.2.1
  - contourpy==1.1.0
  - cycler==0.11.0
  - decorator==4.4.2
  - distlib==0.3.7
  - dm-tree==0.1.8
  - docker-pycreds==0.4.0
  - filelock==3.12.2
  - fonttools==4.41.1
  - frozenlist==1.4.0
  - gitdb==4.0.10
  - gitpython==3.1.32
  - gputil==1.4.0
  - gym==0.23.1
  - gym-notices==0.0.8
  - idna==3.4
  - imageio==2.31.1
  - imageio-ffmpeg==0.4.8
  - jinja2==3.1.2
  - joblib==1.3.1
  - jsonschema==4.18.4
  - jsonschema-specifications==2023.7.1
  - kiwisolver==1.4.4
  - kombu==5.3.1
  - lazy-loader==0.3
  - lz4==4.3.2
  - markupsafe==2.1.3
  - matplotlib==3.7.2
  - moviepy==1.0.3
  - mpmath==1.3.0
  - msgpack==1.0.5
  - networkx==3.1
  - numpy==1.23.5
  - packaging==23.1
```

```
- pandas==2.0.3
- pathtools==0.1.2
- pillow==10.0.0
- platformdirs==3.10.0
- proglog==0.1.10
- prompt-toolkit==3.0.39
- protobuf==4.23.4
- psutil==5.9.5
- pyglet==1.5.27
- pyparsing==3.0.9
- python-dateutil==2.8.2
- pytz==2023.3
- pywavelets==1.4.1
- pyyaml==6.0.1
- ray==2.1.0
- referencing==0.30.0
- requests==2.31.0
- rpds-py==0.9.2
- scikit-image==0.21.0
- scikit-learn==1.3.0
- scipy==1.11.1
- sentry-sdk==1.29.2
- setproctitle==1.3.2
- smmap==5.0.0
- sympy==1.12
- tabulate==0.9.0
- tensorboardx==2.6.2
- threadpoolctl==3.2.0
- tifffile==2023.7.18
- torch==2.0.1
- torch-cluster==1.6.1
- torch-geometric==2.3.1
- torch-scatter==2.1.1
- torch-sparse==0.6.17
- torch-spline-conv==1.2.2
- tqdm==4.65.0
- trainutils==1.1.0
- typing-extensions==4.7.1
- tzdata==2023.3
- urllib3==2.0.4
- vine==5.0.0
- virtualenv==20.24.2
- vmas==1.2.11
- wandb==0.15.8
- wcwidth==0.2.6
```

## Batch size and num\_of\_envs\_per\_worker

```
train_batch_size = 60000
num_workers = 5
num_envs_per_worker = 30
```

```
rollout_fragment_length = (
    train_batch_size // (num_workers * num_envs_per_worker)
)
```

## Torch Ray Library Run Configurations

```
fcnet_model_config = MODEL_DEFAULTS.copy()
fcnet_model_config.update({
    "seed": seed,
    "activation_fn": "relu",
    "share_observations": True,
    "centralised_critic": False,
    "heterogeneous": True,
    "use_beta": False,
    "aggr": "add",
    "topology_type": None,
    "use_mlp": False,
    "add_agent_index": False,
    "trainer": MultiPPOTrainer,
    "share_action_value": True,
    "vf_share_layers": False,
    "trainer": trainer_name,
    "model": {
        "custom_model_config": {
            "dyn_model_hidden_units": 128,
            "dyn_model_layer_num": 2,
            "intr_rew_beta": intr_rew_beta,
        },
    },
})
config = {
    "seed": seed,
    "framework": "torch",
    "env": scenario_name,
    "kl_coeff": 0.01,
    "kl_target": 0.01,
    "lambda": 0.9,
    "clip_param": 0.2,
    "vf_loss_coeff": 1,
    "vf_clip_param": float("inf"),
    "entropy_coeff": 0.01,
    "train_batch_size": train_batch_size,
    "rollout_fragment_length": rollout_fragment_length,
    "sgd_minibatch_size": 4096,
    "num_sgd_iter": 40,
    "num_gpus": int(os.environ.get("RLLIB_NUM_GPUS", "0")),
    "num_workers": num_workers,
    "num_envs_per_worker": num_envs_per_worker,
    "lr": 5e-5,
    "gamma": 0.99,
    "use_gae": True,
```

```

"use_critic": True,
"batch_mode": "complete_episodes",
"model": {
    "custom_model": model_name,
    "custom_action_dist": "hom_multi_action",
    "custom_model_config": {
        "activation_fn": "relu",
        "share_observations": share_observations,
        "gnn_type": "GraphConv",
        "centralised_critic": centralised_critic,
        "heterogeneous": heterogeneous,
        "use_beta": False,
        "aggr": aggr,
        "topology_type": topology_type,
        "use_mlp": use_mlp,
        "add_agent_index": add_agent_index,
        "pos_start": 0,
        "pos_dim": 2,
        "vel_start": 2,
        "vel_dim": 2,
        "goal_rel_start": 4,
        "goal_rel_dim": 2,
        "trainer": trainer_name,
        "share_action_value": share_action_value,
        "alignment_type": alignment_type,
        "comm_radius": comm_radius,
        "dyn_model_hidden_units": dyn_model_hidden_units,
        "dyn_model_layer_num": dyn_model_layer_num,
        "intr_rew_beta": intr_rew_beta,
        "intr_beta_type": intr_beta_type,
        "intr_rew_weighting": intr_rew_weighting,
    }
    if model_name == "GPP0"
    else fcnet_model_config,
},
"dyn_config": {
    "fcnet_hiddens": [128, 128],
    "fcnet_activation": "relu",
    "post_fcnet_hiddens": [],
    "post_fcnet_activation": None,
    "optim_lr": 3e-4,
},
"env_config": {
    "device": "cuda",
    "num_envs": num_envs_per_worker,
    "scenario_name": scenario_name,
    "continuous_actions": continuous_actions,
    "max_steps": max_episode_steps,
    "scenario_config": {
    },
},
},
"evaluation_interval": 20,
"evaluation_duration": 1,

```

```

        "evaluation_num_workers": 1,
        "evaluation_parallel_to_training": True,
        "evaluation_config": {
            "num_envs_per_worker": 1,
            "env_config": {
                "num_envs": 1,
            },
            "callbacks": MultiCallbacks(
                [
                    TrainingUtils.RenderingCallbacks,
                    TrainingUtils.EvaluationCallbacks,
                    TrainingUtils.HeterogeneityMeasureCallbacks,
                ]
            ),
        },
        "callbacks": MultiCallbacks([TrainingUtils.EvaluationCallbacks]),
    }
}

```

## Scenario Configuration Parameters

*# Scenario Configurations for VMAS and MPE Environments*

*# VMAS Flocking*

```

"scenario_config": {
    "n_agents": 4,
    "n_obstacles": 5,
    "min_dist_between_entities": 0.10,
    "dist_shaping_factor": 1,
    "collision_reward": -0.05,
}

```

*# VMAS Navigation*

```

"scenario_config": {
    "n_agents": 4,
    "comm_range": 0.75,
    "shared_rew": True,
    "lidar_range": 0.75,
    "agent_radius": 0.1,
    "final_reward": 1,
    "observe_all_goals": True,
    "pos_shaping_factor": 1,
    "agent_collision_penalty": -0.08
}

```

*# VMAS Sampling*

```

"scenario_config": {
    "n_agents": 3,
    "shared_rew": True,
    "comms_range": 0.50,
    "lidar_range": 0.2,
    "agent_radius": 0.1,
}

```

```

    "collisions": False,
}

# VMAS Joint Passage
"scenario_config": {
    "obs_noise": 0,
    "mass_ratio": 5,
    "n_passages": 1,
    "max_speed_1": None,
    "asym_package": True,
    "joint_length": 0.5,
    "fixed_passage": True,
    "mass_position": 0.75,
    "all_passed_rot": True,
    "use_controller": False,
    "collision_reward": -0.06,
    "random_goal_angle": True,
    "pos_shaping_factor": 1,
    "random_start_angle": True,
    "rot_shaping_factor": 1,
    "energy_reward_coeff": 0,
    "observe_joint_angle": True,
    "joint_angle_obs_noise": 0
}

# MPE Simple Spread
"scenario_config": {
    "n_agents": 4,
    "obs_agents": True,
}

# VMAS Reverse Transport
"scenario_config": {
    "n_agents": 3,
    "package_mass": 1,
    "package_width": 1,
    "package_length": 0.5
}

```
